# Supplementary material for: Three Decades of Formal Methods in Business Process Compliance: A Systematic Literature Review
Source: arXiv:2410.10906 source file (2024-10-13)
Supplement: Supplementary file 1 [file ManualPilotExtraction.pdf]

# Manual Pilot Extraction

| Implementation of RQ | Database | Results | Query | Notes |
|---|---|---|---|---|
| KW1 AND KW2 AND KW3 AND KW4 AND KW5 | | | | |
| ("formal method" OR "formal model" OR "formalism" OR "formal language") AND ( compliance OR conformance OR accordance OR coherence OR enforcement ) AND ( framework OR method OR methodology ) AND ( "Business Process" OR workflow OR "case management" ) AND ( "Regulatory text" OR regulation OR law OR legislation ) | EBSCO | 4 | https://eds.a.ebscohost.com/eds/resultsadvanced?vid=20&sid=fa4543da-0167-490f-9383-26f5950fd373%40sessionmgr4009&bquery=(%22formal+method%22+OR+%22formal+model%22+OR+%22formalism%22+OR+%22formal+language%22)+AND+(compliance+OR+conformance+OR+accordance+OR+coherence+OR+enforcement)+AND+(framework+OR+method+OR+methodology)+AND+(%22Business+Process%22+OR+workflow+OR+%22case+management%22)+AND+(%22Regulatory+text%22+OR+regulation+OR+law+OR+legislation)&bdata=JmNsaTA9UlYmY2x2MD1ZJmNsaTE9RlQxJmNsdjE9WSZjbGkyPURUMSZjbHYyPTE5ODYwMS0yMDE3MTImY2xpMz1MQTk5JmNsdjM9RW5nJnR5cGU9MSZzaXRlPWVkcy1saXZl | No expanders used |
| ("formal method" OR "formal model" OR "formalism" OR "formal language") AND ( compliance OR conformance OR accordance OR coherence OR enforcement ) AND ( framework OR method OR methodology ) AND ( "Business Process" OR workflow OR "case management" ) AND ( "Regulatory text" OR regulation OR law OR legislation ) | EBSCO | 1414 | https://eds.a.ebscohost.com/eds/resultsadvanced?vid=17&sid=fa4543da-0167-490f-9383-26f5950fd373%40sessionmgr4009&bquery=(%22formal+method%22+OR+%22formal+model%22+OR+%22formalism%22+OR+%22formal+language%22)+AND+(compliance+OR+conformance+OR+accordance+OR+coherence+OR+enforcement)+AND+(framework+OR+method+OR+methodology)+AND+(%22Business+Process%22+OR+workflow+OR+%22case+management%22)+AND+(%22Regulatory+text%22+OR+regulation+OR+law+OR+legislation)&bdata=JmNsaTA9UlYmY2x2MD1ZJmNsaTE9RlQxJmNsdjE9WSZjbGkyPURUMSZjbHYyPTE5ODYwMS0yMDE3MTImY2xpMz1MQTk5JmNsdjM9RW5nJnR5cGU9MSZzaXRlPWVkcy1saXZl | Apply "also search within the full text of the articles" |
| TS= (Formal) AND TS= (Compliance OR conformance OR accordance OR coherence OR enforcement) AND TS= (Framework OR method OR methodology) AND TS=("Business Process*" OR workflow* OR "case management") AND TS= ("Regulatory text*" OR regulation* OR law* OR legislation* OR "legal document*" OR policy OR policies OR legal) | WOS | 17 | http://apps.webofknowledge.com.proxy.findit.dtu.dk/Search.do?product=WOS&SID=Y2ZXq2XQ8dV43Qz3jFZ&search_mode=GeneralSearch&prID=2a7c432b-a9cf-4fbc-8f3c-426983f1ef32 | Applying exclusion cirteria for considering only articles reduces dataset to 16 entries |
| ALL ( ( "Formal method" ) AND ( compliance OR conformance OR accordance OR coherence OR enforcement ) AND ( framework OR method OR methodology ) AND ( "Business Process*" OR workflow* OR "case management" ) AND ( "Regulatory text*" OR regulation* OR law* OR legislation* ) ) | Scopus | 145 | https://www-scopus-com.proxy.findit.dtu.dk/results/results.uri?numberOfFields=0&src=s&clickedLink=&edit=t&editSaveSearch=&origin=searchbasic&authorTab=&affiliationTab=&advancedTab=&scint=1&menu=search&tablin=&searchterm1=%28%22Formal+method%22%29+AND+%28Compliance+OR+conformance+OR+accordance+OR+coherence+OR+enforcement%29+AND+%28Framework+OR+method+OR+methodology%29+AND+%28%22Business+Process*%22+OR+workflow*+OR+%22case+management%22%29+AND+%28%22Regulatory+text*%22+OR+regulation*+OR+law*+OR+legislation*%29&field1=ALL&dateType=Publication_Date_Type&yearFrom=1986&yearTo=Present&loadDate=7&documenttype=All&resetFormLink=&st1=%28%22Formal+method%22%29+AND+%28Compliance+OR+conformance+OR+accordance+OR+coherence+OR+enforcement%29+AND+%28Framework+OR+method+OR+methodology%29+AND+%28%22Business+Process*%22+OR+workflow*+OR+%22case+management%22%29+AND+%28%22Regulatory+text*%22+OR+regulation*+OR+law*+OR+legislation*%29&st2=&sot=b&sdt=b&sl=261&s=ALL%28%28%22Formal+method%22%29+AND+%28Compliance+OR+conformance+OR+accordance+OR+coherence+OR+enforcement%29+AND+%28Framework+OR+method+OR+methodology%29+AND+%28%22Business+Process*%22+OR+workflow*+OR+%22case+management%22%29+AND+%28%22Regulatory+text*%22+OR+regulation*+OR+law*+OR+legislation*%29%29&sid=8b9012f09a0d97b62c4b74abbb1b7e3d&searchId=8b9012f09a0d97b62c4b74abbb1b7e3d&txGid=55cd3d39926687e84638ed5436bb14f7&sort=plf-f&originationType=b&rr= | Reached the search string limit |
| ALL ( ( "Formal model" ) AND ( compliance OR conformance OR accordance OR coherence OR enforcement ) AND ( framework OR method OR methodology ) AND ( "Business Process*" OR workflow* OR "case management" ) AND ( "Regulatory text*" OR regulation* OR law* OR legislation* ) ) | Scopus | 64 | https://www-scopus-com.proxy.findit.dtu.dk/results/results.uri?numberOfFields=0&src=s&clickedLink=&edit=t&editSaveSearch=&origin=searchbasic&authorTab=&affiliationTab=&advancedTab=&scint=1&menu=search&tablin=&searchterm1=%28%22Formal+model%22%29+AND+%28Compliance+OR+conformance+OR+accordance+OR+coherence+OR+enforcement%29+AND+%28Framework+OR+method+OR+methodology%29+AND+%28%22Business+Process*%22+OR+workflow*+OR+%22case+management%22%29+AND+%28%22Regulatory+text*%22+OR+regulation*+OR+law*+OR+legislation*%29&field1=ALL&dateType=Publication_Date_Type&yearFrom=1986&yearTo=Present&loadDate=7&documenttype=All&resetFormLink=&st1=%28%22Formal+model%22%29+AND+%28Compliance+OR+conformance+OR+accordance+OR+coherence+OR+enforcement%29+AND+%28Framework+OR+method+OR+methodology%29+AND+%28%22Business+Process*%22+OR+workflow*+OR+%22case+management%22%29+AND+%28%22Regulatory+text*%22+OR+regulation*+OR+law*+OR+legislation*%29&st2=&sot=b&sdt=b&sl=260&s=ALL%28%28%22Formal+model%22%29+AND+%28Compliance+OR+conformance+OR+accordance+OR+coherence+OR+enforcement%29+AND+%28Framework+OR+method+OR+methodology%29+AND+%28%22Business+Process*%22+OR+workflow*+OR+%22case+management%22%29+AND+%28%22Regulatory+text*%22+OR+regulation*+OR+law*+OR+legislation*%29%29&sid=8b9012f09a0d97b62c4b74abbb1b7e3d&searchId=8b9012f09a0d97b62c4b74abbb1b7e3d&txGid=55cd3d39926687e84638ed5436bb14f7&sort=plf-f&originationType=b&rr= | Reached the search string limit |

| | | | | |
|---|---|---|---|---|
| ALL ( ( "Formalism" ) AND ( compliance OR conformance OR accordance OR coherence OR enforcement ) AND ( framework OR method OR methodology ) AND ( "Business Process*" OR workflow* OR "case management" ) AND ( "Regulatory text*" OR regulation* OR law* OR legislation* ) ) | Scopus | 125 | https://www-scopus-com.proxy.findit.dtu.dk/results/results.uri?numberOfFields=0&src=s&clickedLink=&edit=t&editSaveSearch=&origin=searchbasic&authorTab=&affiliationTab=&advancedTab=&scint=1&menu=search&tablin=&searchterm1=%28%22Formalism%22%29+AND+%28Compliance+OR+conformance+OR+accordance+OR+coherence+OR+enforcement%29+AND+%28Framework+OR+method+OR+methodology%29+AND+%28%22Business+Process*%22+OR+workflow*+OR+%22case+management%22%29+AND+%28%22Regulatory+text*%22+OR+regulation*+OR+law*+OR+legislation*%29&field1=ALL&dateType=Publication_Date_Type&yearFrom=1986&yearTo=Present&loadDate=7&documenttype=All&resetFormLink=&st1=%28%22Formalism%22%29+AND+%28Compliance+OR+conformance+OR+accordance+OR+coherence+OR+enforcement%29+AND+%28Framework+OR+method+OR+methodology%29+AND+%28%22Business+Process*%22+OR+workflow*+OR+%22case+management%22%29+AND+%28%22Regulatory+text*%22+OR+regulation*+OR+law*+OR+legislation*%29&st2=&sot=b&sdt=b&sl=257&s=ALL%28%28%22Formalism%22%29+AND+%28Compliance+OR+conformance+OR+accordance+OR+coherence+OR+enforcement%29+AND+%28Framework+OR+method+OR+methodology%29+AND+%28%22Business+Process*%22+OR+workflow*+OR+%22case+management%22%29+AND+%28%22Regulatory+text*%22+OR+regulation*+OR+law*+OR+legislation*%29%29&sid=8b9012f09a0d97b62c4b74abbb1b7e3d&searchId=8b9012f09a0d97b62c4b74abbb1b7e3d&txGid=55cd3d39926687e84638ed5436bb14f7&sort=plf-f&originationType=b&rr= | Reached the search string limit |
| ALL ( ( "Formal language" ) AND ( compliance OR conformance OR accordance OR coherence OR enforcement ) AND ( framework OR method OR methodology ) AND ( "Business Process" OR workflow OR "case management" ) AND ( "Regulatory text*" OR regulation* OR law* OR legislation* ) ) | Scopus | 41 | https://www-scopus-com.proxy.findit.dtu.dk/results/results.uri?numberOfFields=0&src=s&clickedLink=&edit=t&editSaveSearch=&origin=searchbasic&authorTab=&affiliationTab=&advancedTab=&scint=1&menu=search&tablin=&searchterm1=%28%22Formal+language%22%29+AND+%28Compliance+OR+conformance+OR+accordance+OR+coherence+OR+enforcement%29+AND+%28Framework+OR+method+OR+methodology%29+AND+%28%22Business+Process%22+OR+workflow+OR+%22case+management%22%29+AND+%28%22Regulatory+text*%22+OR+regulation*+OR+law*+OR+legislation*%29&field1=ALL&dateType=Publication_Date_Type&yearFrom=1986&yearTo=Present&loadDate=7&documenttype=All&resetFormLink=&st1=%28%22Formal+language%22%29+AND+%28Compliance+OR+conformance+OR+accordance+OR+coherence+OR+enforcement%29+AND+%28Framework+OR+method+OR+methodology%29+AND+%28%22Business+Process%22+OR+workflow+OR+%22case+management%22%29+AND+%28%22Regulatory+text*%22+OR+regulation*+OR+law*+OR+legislation*%29&st2=&sot=b&sdt=b&sl=261&s=ALL%28%28%22Formal+language%22%29+AND+%28Compliance+OR+conformance+OR+accordance+OR+coherence+OR+enforcement%29+AND+%28Framework+OR+method+OR+methodology%29+AND+%28%22Business+Process%22+OR+workflow+OR+%22case+management%22%29+AND+%28%22Regulatory+text*%22+OR+regulation*+OR+law*+OR+legislation*%29%29&sid=8b9012f09a0d97b62c4b74abbb1b7e3d&searchId=8b9012f09a0d97b62c4b74abbb1b7e3d&txGid=55cd3d39926687e84638ed5436bb14f7&sort=plf-f&originationType=b&rr= | Reached the search string limit |
| ("formal method" OR "formal model" OR "formalism" OR "formal language") AND ( compliance OR conformance OR accordance OR coherence OR enforcement ) AND ( framework OR method OR methodology ) AND ( "Business Process" OR workflow OR "case management" ) AND ( "Regulatory text" OR regulation OR law OR legislation ) | ScienceDirect | 765 | http://www.sciencedirect.com.proxy.findit.dtu.dk/science?_ob=ArticleListURL&_method=list&_ArticleListID=-1240825824&_sort=r&_st=5&md5=dd90f4f41c9dbd3208286208d8e9feb7&searchtype=a | [All Sources(Business, Management and Accounting,Computer Science,Decision Sciences,Economics, Econometrics and Finance,Engineering,Mathematics,Nursing and Health Professions,Philosophy)]. |
| formal AND ( compliance OR conformance OR accordance OR coherence OR enforcement ) AND ( framework OR method OR methodology ) AND ( "Business Process" OR workflow OR "case management" ) AND (regulation) | Xplore | 6 | http://ieeexplore.ieee.org.proxy.findit.dtu.dk/search/searchresult.jsp?action=search&sortType=&rowsPerPage=&matchBoolean=true&searchField=Search_All&queryText=(formal AND ( compliance OR conformance OR accordance OR coherence OR enforcement ) AND ( framework OR method OR methodology ) AND ( .QT.Business Process*.QT. OR workflow* OR .QT.case management.QT. ) AND (regulation*) )&newsearch=true | Search engine allows up to 15 terms |
| formal AND ( compliance OR conformance OR accordance OR coherence OR enforcement ) AND ( framework OR method OR methodology ) AND ( "Business Process" OR workflow OR "case management" ) AND (law ) | Xplore | 6 | http://ieeexplore.ieee.org.proxy.findit.dtu.dk/search/searchresult.jsp?action=search&sortType=&rowsPerPage=&matchBoolean=true&searchField=Search_All&queryText=(formal AND ( compliance OR conformance OR accordance OR coherence OR enforcement ) AND ( framework OR method OR methodology ) AND ( .QT.Business Process*.QT. OR workflow* OR .QT.case management.QT. ) AND (law*) )&newsearch=true | Search engine allows up to 15 terms |
| formal AND ( compliance OR conformance OR accordance OR coherence OR enforcement ) AND ( framework OR method OR methodology ) AND ( "Business Process" OR workflow OR "case management" ) AND (legislation ) | Xplore | 1 | http://ieeexplore.ieee.org.proxy.findit.dtu.dk/search/searchresult.jsp?action=search&sortType=&rowsPerPage=&matchBoolean=true&searchField=Search_All&queryText=(formal AND ( compliance OR conformance OR accordance OR coherence OR enforcement ) AND ( framework OR method OR methodology ) AND ( .QT.Business Process*.QT. OR workflow* OR .QT.case management.QT. ) AND (legislation*) )&newsearch=true | Search engine allows up to 15 terms |
| ("formal method" OR "formal model" OR "formalism" OR "formal language") AND ( compliance OR conformance OR accordance OR coherence OR enforcement ) AND ( framework OR methodology ) AND ( "Business Process" OR workflow OR "case management" ) AND ( "Regulatory text" OR regulation OR law OR legislation ) | Springerlink | 655 | https://link-springer-com.proxy.findit.dtu.dk/search?query=%28%22formal+method%22+OR+%22formal+model%22+OR+%22formalism%22+OR+%22formal+language%22%29+AND+%28+compliance+OR+conformance+OR+accordance+OR+coherence+OR+enforcement+%29+AND+%28+framework+OR+methodology+%29+AND+%28+%22Business+Process%22+OR+workflow+OR+%22case+management%22+%29+AND+%28+%22Regulatory+text%22+OR+regulation+OR+law+OR+legislation+%29+&facet-language=%22En%22&date-facet-mode=between&facet-end-year=2017&showAll=false&facet-start-year=1986 | Only searches full-text (no title+abstract search allowed) --- Apply limit criteria to **only include conference papers** |

| | | | | |
|---|---|---|---|---|
| ("formal method" OR "formal model" OR "formalism" OR "formal language") AND ( compliance OR conformance OR accordance OR coherence OR enforcement ) AND ( framework OR methodology ) AND ( "Business Process" OR workflow OR "case management" ) AND ( "Regulatory text" OR regulation OR law OR legislation ) | Springerlink | 1676 | https://link-springer-com.proxy.findit.dtu.dk/search?query=%28%22formal+method%22+OR+%22formal+model%22+OR+%22formalism%22+OR+%22formal+language%22%29+AND+%28+compliance+OR+conformance+OR+accordance+OR+coherence+OR+enforcement+%29+AND+%28+framework+OR+methodology+%29+AND+%28+%22Business+Process%22+OR+workflow+OR+%22case+management%22+%29+AND+%28+%22Regulatory+text%22+OR+regulation+OR+law+OR+legislation+%29+&facet-language=%22En%22&date-facet-mode=between&facet-end-year=2017&showAll=false&facet-start-year=1986 | Only searches full-text (no title+abstract search allowed) |
| ("formal model" "formal method" formalism "formal language") AND (compliance conformance accordance coherence enforcement) AND ( framework methodology) AND ("Business Process" workflow "case management") AND ("Regulatory text" regulation law legislation) | ACM DL | 10 | https://dl-acm-org.proxy.findit.dtu.dk/results.cfm?query=(%22formal%20model%22%20%22formal%20method%22%20formalism%20%22formal%20language%22)%20AND%20(compliance%20conformance%20accordance%20coherence%20enforcement)%20AND%20(%20framework%20methodology)%20AND%20(%22Business%20Process%22%20workflow%20%22case%20management%22)%20AND%20(%22Regulatory%20text%22%20regulation%20law%20legislation)&within=owners.owner=HOSTED&filtered=&dte=&bfr= | |
| formal  AND ( compliance OR conformance OR accordance OR coherence OR enforcement ) AND ( framework OR method OR methodology ) AND ( "Business Process" OR workflow OR "case management" ) AND ( "Regulatory text" OR regulation OR law OR legislation ) | JST | 87 | https://www.jstor.org/action/doBasicSearch?searchType=facetSearch&page=1&sd=1986&ed=2017&facet_business-discipline=YnVzaW5lc3MtZGlzY2lwbGluZQ%3D%3D&facet_education-discipline=ZWR1Y2F0aW9uLWRpc2NpcGxpbmU%3D&facet_finance-discipline=ZmluYW5jZS1kaXNjaXBsaW5l&facet_healthsciences-discipline=aGVhbHRoc2NpZW5jZXMtZGlzY2lwbGluZQ%3D%3D&facet_law-discipline=bGF3LWRpc2NpcGxpbmU%3D&facet_manorgbeha-discipline=bWFub3JnYmVoYS1kaXNjaXBsaW5l&facet_philosophy-discipline=cGhpbG9zb3BoeS1kaXNjaXBsaW5l&facet_politicalscience-discipline=cG9saXRpY2Fsc2NpZW5jZS1kaXNjaXBsaW5l&facet_technology-discipline=dGVjaG5vbG9neS1kaXNjaXBsaW5l&Query=formal+++AND++%28+compliance++OR++conformance++OR++accordance++OR++coherence++OR++enforcement+%29++AND++%28+framework++OR++method++OR++methodology+%29++AND++%28+%22Business+Process%22++OR++workflow++OR++%22case+management%22+%29++AND++%28+%22Regulatory+text%22++OR++regulation++OR++law++OR++legislation+%29+ | Use the word "formal" instead of the keywords to abide to the space limitation of jstor wrt size of the query |
| formal AND ( compliance OR conformance OR accordance OR coherence OR enforcement ) AND ( framework OR method OR methodology ) AND ( "Business Process" OR workflow OR "case management" ) AND ( "Regulatory text" OR regulation OR law OR legislation ) | BSP | 2 | http://web.b.ebscohost.com.proxy.findit.dtu.dk/ehost/resultsadvanced?vid=2&sid=ee4a84ea-844e-48c3-87aa-7c41b9054006%40sessionmgr101&bquery=formal+AND+(compliance+OR+conformance+OR+accordance+OR+coherence+OR+enforcement)+AND+(framework+OR+method+OR+methodology)+AND+(%22Business+Process%22+OR+workflow+OR+%22case+management%22)+AND+(%22Regulatory+text%22+OR+regulation+OR+law+OR+legislation)&bdata=JmRiPWJ1aCZ0eXBlPTEmc2l0ZT1laG9zdC1saXZl | Use the word "formal" instead of the keywords to abide to the space limitation of BSP wrt size of the query |
